# Supplementary material for: Policy Optimization in Adversarial MDPs: Improved Exploration via Dilated Bonuses
Source: arXiv:2107.08346 source file (2021-07-18)
Supplement: Supplementary file 1 [file appendix-linearQ-exploratory.tex]

%!TEX root=main.tex
\section{Details for Linear-$Q$ with a Simulator and an Exploratory Policy}

The main algorithm (\pref{alg: linear Q with exploratory}) follows the same idea as \pref{alg: linear Q}. The main difference is that we can leverage $\pi_0$ to perform exploration. To do so, in Step 1 of the algorithm, we draw a Bernoulli random variable $Y_t\sim \textsc{Bernoulli}(\explore)$ (for some $\explore\in(0,1)$) to indicate whether in this round the learner should use $\pi_0$. If $Y_t$ is $1$, then the learner further randomly draw $h_t^*$ from $0, \ldots, H-1$. Then she walks from $x_0$ to layer $h_t^*$ using $\pi_0$, and then continues with $\pi_t$ to the end. In this way, the learner can explicitly explore the state space on every layer, which facilitates estimating $\theta_{t,h}^{\pi_t}$ with less bias. 

Because we mix the exploration into the policy, we perform a slightly different procedure $\GRMIX$ in Step 2, which does not incorporate the $\gamma$ parameter as in $\GR$. Instead, it will estimate the inverse of $\cov_{t,h}^{\mix}=(1-\explore) \cov_{t,h} + \explore \cov_{h}^{\pi_0}$ where $\cov_{t,h}$ is the covariance matrix under $\pi_t$ and $\cov_{h}^{\pi_0}$ is the covariance matrix under $\pi_0$.  

The new construction of $\hattheta_{t,h}$ in Step 3 makes it an estimator of $\theta_{t,h}^{\pi_t}$ with low error. To see this, observe that
\begin{align}
    %&\E_t\left[\hattheta_{t,h}\right] \nonumber\\
    &\E_t\left[\left( (1-Y_t)+Y_t H\ind[h=h_t^*]\right)\phi(x_{t,h}, a_{t,h})L_{t,h} \right] \nonumber\\
    &= \explore  \E_t\left[H\ind[h=h_t^*]\phi(x_{t,h}, a_{t,h})L_{t,h} ~|~ Y_t=1\right] + (1-\explore)\E_t\left[\phi(x_{t,h}, a_{t,h})L_{t,h} ~\big|~ Y_t=0\right] \nonumber\\
    &= \explore  \E_t\left[H\ind[h=h_t^*]\phi(x_{t,h}, a_{t,h})\phi(x_{t,h}, a_{t,h})^\top \theta_{t,h}^{\pi_t} ~\big|~ Y_t=1\right] \nonumber\\
    &\qquad \qquad + (1-\explore)\E_t\left[\phi(x_{t,h}, a_{t,h})\phi(x_{t,h}, a_{t,h})^\top \theta_{t,h}^{\pi_t} ~\big|~ Y_t=0\right] \nonumber\\
    &=\explore  \E_t\left[H\ind[h=h_t^*]\right]\cov_{h}^{\pi_0} \theta_{t,h}^{\pi_t}   
    + (1-\explore)\E_t\left[\cov_{t,h} \theta_{t,h}^{\pi_t}\right] \nonumber\\
    &=\left(\explore\cov_{h}^{\pi_0} + (1-\explore)\cov_{t,h}\right) \theta_{t,h}^{\pi_t}   \nonumber\\
    &= \cov_{t,h}^{\mix}\theta_{t,h}^{\pi_t} \label{eq:linear-Q_expectation} 
    %&\approx  \theta_{t,h}^{\pi_t}, \nonumber
\end{align} 
and thus 
\[
\E_t\left[\hattheta_{t,h}\right] = \E_t\left[\hatcov_{t,h}\left( (1-Y_t)+Y_t H\ind[h=h_t^*]\right)\phi(x_{t,h}, a_{t,h})L_{t,h} \right] = \E_t\left[\hatcov_{t,h}\right]\cov_{t,h}^{\mix}\theta_{t,h}^{\pi_t} \approx  \theta_{t,h}^{\pi_t},
\]
%\begin{align}
%    &\E_t\left[\hattheta_{t,h}\right] \nonumber\\
%    &= \E_t\left[\hatcov_{t,h}\left( (1-Y_t)+Y_t H\ind[h=h_t^*]\right)\phi(x_{t,h}, a_{t,h})L_{t,h} \right] \nonumber\\
%    &= \explore  \E_t\left[H\ind[h=h_t^*]\hatcov_{t,h}\phi(x_{t,h}, a_{t,h})L_{t,h} ~|~ Y_t=1\right] + (1-\explore)\E_t\left[\hatcov_{t,h}\phi(x_{t,h}, a_{t,h})L_{t,h} ~\big|~ Y_t=0\right] \nonumber\\
%    &= \explore  \E_t\left[H\ind[h=h_t^*]\hatcov_{t,h}\phi(x_{t,h}, a_{t,h})\phi(x_{t,h}, a_{t,h})^\top \theta_{t,h}^{\pi_t} ~\big|~ Y_t=1\right] \nonumber\\
%    &\qquad \qquad + (1-\explore)\E_t\left[\hatcov_{t,h}\phi(x_{t,h}, a_{t,h})\phi(x_{t,h}, a_{t,h})^\top \theta_{t,h}^{\pi_t} ~\big|~ Y_t=0\right] \nonumber\\
%    &=\explore  \E_t\left[H\ind[h=h_t^*]\right]\hatcov_{t,h}\cov_{h}^{\pi_0} \theta_{t,h}^{\pi_t}   
%    + (1-\explore)\E_t\left[\hatcov_{t,h}\cov_{t,h} \theta_{t,h}^{\pi_t}\right] \nonumber\\
%    &=\hatcov_{t,h}\left(\explore\cov_{h}^{\pi_0} + (1-\explore)\cov_{t,h}\right) \theta_{t,h}^{\pi_t}   \nonumber\\
%    &= \hatcov_{t,h}\cov_{t,h}^{\mix}\theta_{t,h}^{\pi_t} \nonumber\\
%    &\approx  \theta_{t,h}^{\pi_t}, \nonumber
%\end{align} 
where the last step is because $\hatcov_{t,h}$ is approximately the inverse of $\cov_{t,h}^{\mix}$.

In \pref{app: grmix analysis}, we first present the algorithm \GRMIX and its analysis (similar to \pref{lem: GR lemma contingency}). Then in \pref{app: regret analysis mix}, we perform regret analysis for \pref{alg: linear Q with exploratory}. 

\begin{algorithm}[t]
    \caption{Policy Optimization with Dilated Bonuses (Linear-$Q$ Case with an Exploratory Policy)}
    \label{alg: linear Q with exploratory}
    \textbf{parameters}: $\lambda_{\min}, \beta, \eta, \epsilon, \explore$,  $M=\left\lceil\frac{96\ln(dHT)\ln^2(\frac{1}{\epsilon\explore\lambda_{\min}})}{\epsilon^2\explore^2\lambda_{\min}^2}\right\rceil$, $N=\left\lceil\frac{2}{\explore\lambda_{\min}}\ln \frac{1}{\epsilon \explore \lambda_{\min}}\right\rceil$.  \\ 
    \For{$t=1,2,\ldots, T$}{
        \textbf{Step 1: Interact with the environment.} 
        Let $\pi_t$ be defined such that for each $x\in X_h$,
        \begin{align}
              \pi_t(a|x) \propto \exp\left( -\eta  \sum_{\tau=1}^{t-1}\left(\phi(x,a)^\top \hattheta_{\tau, h}   - \Bonus(\tau,x,a)\right) \right).  
        \end{align} 
        
        Draw $Y_t\sim \textsc{Bernoulli}(\explore)$. \\
        \If{$Y_t=1$}{
            Draw $h_t^* \sim \text{Uniform}\{0, \ldots, H-1\}$. \\
            Execute $\pi_0$ in steps $0,\ldots, h_t^*-1$; continue with $\pi_t$ in steps $h_t^*, \ldots, H-1$. 
        }
        \lElse{
            Execute $\pi_t$. 
        }
        \ \\
        Obtain trajectory $\{(x_{t,h}, a_{t,h}, \ell_t(x_{t,h}, a_{t,h}))\}_{h=0}^{H-1}$.  
        \ \\
        \ \\
        \textbf{Step 2: Construct covariance matrix inverse estimators.}  
        \begin{align*} 
             \left\{\hatcov_{t, h}\right\}_{h=0}^{H-1} = \GRMIX\left(t, M, N\right).   \tag{see \pref{alg: GRMIX}} 
        \end{align*}
        %Specially, in $\GR$, we estimate $\left(\explore \cov_{h}^{\pi_0} + (1-\explore)\cov_h^{\pi_t} \right)^{-1}$. \\
        \ \\ 
        \textbf{Step 3: Construct $Q$-function weight estimators.} For all $h = 0, \ldots, H-1$,
%        \If{$Y_t=0$}{
            \begin{align*}
           \hattheta_{t, h}&= \hatcov_{t,h}\left((1-Y_t) + Y_tH\ind[h=h_t^*]\right)\phi(x_{t,h}, a_{t,h})L_{t,h}, \quad \text{where\ } L_{t,h}= \sum_{i=h}^{H-1}\ell_t(x_{t,i},a_{t,i}).
            \end{align*}
%        }
%        \Else{
%            \begin{align}
%                \hattheta_{t, h}&=
%                \begin{cases}
%                    H\hatcov_{t,h} \phi(x_{t,h},a_{t,h})L_{t,h}  &\text{if\ } h=h_t^*, \\
%                    0 &\text{else.}
%                \end{cases}
%            \end{align}
%        }
    }
\end{algorithm}

\subsection{\GRMIX} 
\label{app: grmix analysis}
\begin{algorithm}
    \caption{$\GRMIX(t, M, N)$}
    \label{alg: GRMIX}
    Let $c=\frac{1}{2}$. \\
    \For{$m=1, \ldots, M$}{
    \For{$n=1,\ldots, N$}{
            With probability $1-\explore$, generate path $(x_{n,0},a_{n,0}),\ldots, (x_{n,H-1}, a_{n,H-1})$ using $\pi_t$; otherwise, generate it using $\pi_0$. \\ 
            For all $h$, compute $Y_{n,h}= \phi(x_{n,h},a_{n,h})\phi(x_{n,h},a_{n,h})^\top$.\\
            For all $h$, compute 
            $Z_{n,h}=\Pi_{j=1}^{n}(I-cY_{j,h})$.
        }
        For all $h$, set $\hatcovk_{t,h} = cI + c\sum_{n=1}^N Z_{n,h}$.   
    }
    For all $h$, set $\hatcov_{t,h} = \frac{1}{M}\sum_{m=1}^M \hatcovk_{t,h}$.\\
    \textbf{return} $\hatcov_{t,h}$ for all $h=0,\ldots, H-1$.  
\end{algorithm}

\begin{lemma}
    \label{lem: GR lemma contingency exploratory}
    Let $M=\left\lceil\frac{96\ln(dHT)\ln^2(\frac{1}{\epsilon\explore\lambda})}{\epsilon^2\explore^2\lambda^2}\right\rceil$, $N=\left\lceil\frac{2}{\explore\lambda}\ln \frac{1}{\epsilon\explore \lambda}\right\rceil$ for some $\epsilon>0$. Let $\cov_{t,h}=\E_{\pi_t}[\phi(x_h,a_h)\phi(x_h,a_h)^\top]$ and $\cov_h^{\pi_0} = \E_{\pi_0}[\phi(x_h,a_h)\phi(x_h,a_h)^\top]$ and $\cov_{t,h}^{\mix} = (1-\explore)\cov_{t,h} + \explore\cov_{h}^{\pi_0}$. Suppose that $\lambda>0$ is a lower bound for the minimum eigenvalue of $\cov_h^{\pi_0}$. Then $\GRMIX$ (\pref{alg: GRMIX}) with input $(t,M,N)$ ensures the following for all $h$: %with probability at least $1-\frac{1}{T^3}$, the following hold for all $h$: 
    \begin{align}
        \norm{\hatcov_{t,h}}_{\text{\rm op}} &\leq \frac{2}{\explore\lambda}\ln \frac{1}{\epsilon\explore\lambda}. \label{eq: GE 13} \\  
        \norm{\E_t\left[\hatcov_{t,h}\right] - (\cov_{t,h}^{\mix})^{-1}}_{\text{\rm op}} &\leq \epsilon, \label{eq: GE 15}\\
        \norm{\hatcov_{t,h} -  (\cov_{t,h}^{\mix})^{-1}}_{\text{\rm op}} &\leq 2\epsilon. \label{eq: GE 14} \\
        \norm{\hatcov_{t,h}\cov_{t,h}^{\mix}}_{\text{\rm op}}
        &\leq 1 + 2\epsilon,  \label{eq: bounded norm prod exploratory}
    \end{align} 
        where $\norm{\cdot}_{\text{\rm op}}$ represents the spectral norm and the last two properties \pref{eq: GE 14} and \pref{eq: bounded norm prod exploratory} hold with probability at least $1-\frac{1}{T^3}$.
\end{lemma}
\begin{proof}

To prove \pref{eq: GE 13}, notice that each one of $\hatcovk_{t,h}$, $m=1,\ldots, M$, is a sum of $N+1$ terms. Furthermore, the $n$-th term of them ($cZ_{n,h}$ in \pref{alg: GRMIX}) has an operator norm upper bounded by $c$. Therefore, 
\begin{align*}
    \norm{\hatcovk_{t,h}}_{\text{op}} \leq c(N+1) = \frac{1}{2}(N+1) \leq \frac{2}{\explore\lambda}\ln \frac{1}{\epsilon\explore\lambda}.  
\end{align*}
Since $\hatcov_{t,h}$ is an average of $\hatcovk_{t,h}$, this implies \pref{eq: GE 13}. 

To show \pref{eq: GE 15}, observe that
\begin{align*}
    \E_t\left[\hatcov_{t,h}\right] = \E_t\left[\hatcovk_{t,h}\right]
    &= cI + c\sum_{i=1}^N \left(I-c \cov_{t,h}^{\mix}\right)^i \\
    &= {(\cov_{t,h}^{\mix})}^{-1} \left( I - \left(I - c \cov_{t,h}^{\mix}\right)^{N+1} \right) 
\end{align*}
where we use the formula: $ \left(I+\sum_{i=1}^{N}A^{i}\right) = (I-A)^{-1}(I-A^{N+1})$ with $A=I-c\cov_{t,h}^{\mix}$.

Thus, 
\begin{align*}
    \norm{\E_t\left[\hatcov_{t,h}\right] - (\cov_{t,h}^{\mix})^{-1}}_{\text{op}} 
    &= \norm{\left(\cov_{t,h}^{\mix}\right)^{-1}\left(I - c \cov_{t,h}^{\mix}\right)^{N+1}}_{\text{op}} \\
    &\leq \frac{(1-c\explore\lambda)^{N+1}}{\explore\lambda}  \leq \frac{e^{-(N+1)c\explore\lambda}}{\explore\lambda} \leq \epsilon,
\end{align*}
where the last inequality is by our choice of $N$ and that $c=\frac{1}{2}$. 

To show \pref{eq: GE 14}, we only further need 
\begin{align*}
    \norm{\hatcov_{t,h} - \E_t\left[\hatcov_{t,h}\right]}_{\text{op}}\leq \epsilon
\end{align*}
and combine it with \pref{eq: GE 15}. 
This can be shown by applying \pref{lem: matrix azuma} with $X_k = \widehat{\Sigma}^{+(k)}_{t,h}, \sigma=\frac{2}{\explore\lambda}\ln \frac{1}{\epsilon\explore\lambda}$, $\tau=\epsilon$, and $n=M$ (see the proof for \pref{eq: GE 4} for the reason). This gives the following statement: the event $\norm{\hatcov_{t,h} - \E_t\left[\hatcov_{t,h}\right]}_{\text{op}}> \epsilon$ holds with probability less than
\begin{align*}
    d\exp\left(-M \times \epsilon^2 \times \frac{1}{8}\times \frac{\explore^2\lambda^2}{4\ln^2\frac{1}{\epsilon\explore\lambda}}\right)\leq \frac{1}{d^2H^3T^3} \leq \frac{1}{HT^3}
\end{align*}
by our choice of $M$. The conclusion follows by a union bound over $h$. 

To prove \pref{eq: bounded norm prod exploratory}, observe that with \pref{eq: GE 14}, we have 
\begin{align*}
    \norm{\hatcov_{t,h} \cov_{t,h}^{\mix}}_{\text{op}}
    &\leq  \norm{(\cov_{t,h}^{\mix})^{-1} \cov_{t,h}^{\mix}}_{\text{op}} + \norm{\left(\hatcov_{t,h} - (\cov_{t,h}^{\mix})^{-1}\right) \cov_{t,h}^{\mix}}_{\text{op}} 
    \leq 1 + 2\epsilon
\end{align*}
since $\norm{\cov_{t,h}^{\mix}}_{\text{op}}\leq 1$. 
%Notice that 
%\begin{align*}
%    \norm{ \left(I-c\left(\gamma I + \cov_t\right)\right)^N}_{\text{op}}\leq (1-c\gamma)^N \leq \exp\left(-Nc\gamma\right). 
%\end{align*}
%Making this smaller than $\epsilon$ requires $N=\widetilde{\Theta}\left( \frac{1}{c\gamma}\log(1/\epsilon) \right)$. 
\end{proof}

\subsection{Regret Analysis}
\label{app: regret analysis mix}

The analysis follows the same outline discussed in \pref{sec:linear-Q-analysis}.
In particular, we define $\bonusQ_t(x,a)$ for all $t,x,a$ again using the same virtual process,
and then we follow the same regret decomposition as in \pref{eq:decompose tabular regret}, with $\Qht_t(x,a)\triangleq \phi(x,a)^\top \hattheta_{t,h}$ (for $x \in X_h$).
We then bound $\E[\bias + \biastwo]$ and $\E[\regterm]$ in \pref{lem: mix algorithm bias term} and \pref{lem: E.3 lemma} respectively.

\begin{lemma}\label{lem: mix algorithm bias term}
$
         \E[\bias + \biastwo] = \order(\epsilon H^3 T).
$
\end{lemma}

\begin{proof}
    Consider a specific $(t,x,a)$. Let $h$ be such that $x\in X_h$. Then we have
    \begin{align*}
        &\E_t\left[Q^{\pi_t}_t(x,a) - \Qht_t(x,a)\right]  \nonumber  \\
        &=\phi(x,a)^\top \left(\theta_{t,h}^{\pi_t} - \E_t\left[\hattheta_{t,h}\right]\right) \nonumber \\ 
        %&= \phi(x,a)^\top \left(\theta_{t,h}^{\pi_t} - \E_t\left[\hatcov_{t,h}\right]\E_t\left[ \phi(x_{t,h},a_{t,h})L_{t,h} \right]\right) \nonumber \\
        &=  \phi(x,a)^\top \left(\theta_{t,h}^{\pi_t} -  \E_t\left[\hatcov_{t,h}\right]\E_t\left[  \Big((1-Y_t) + Y_t\ind[h_t^*=h]H\Big)\phi(x_{t,h},a_{t,h})L_{t,h} \right]\right)  + \order(\epsilon H^2) \\
        &=  \phi(x,a)^\top \left(\theta_{t,h}^{\pi_t} -  (\cov_{t,h}^{\mix})^{-1}\E_t\left[  \Big((1-Y_t) + Y_t\ind[h_t^*=h]H\Big)\phi(x_{t,h},a_{t,h})L_{t,h} \right]\right)  + \order(\epsilon H^2)  \tag{by \pref{lem: GR lemma contingency exploratory} and that $\|\phi(x,a)\|\leq 1$ for all $x,a$ and $L_{t,h}\leq H$} \\
        &= \phi(x,a)^\top \left(\theta_{t,h}^{\pi_t} -  (\cov_{t,h}^{\mix})^{-1}\cov_{t,h}^{\mix} \theta_{t,h}^{\pi_t}\right) + \order(\epsilon H^2) \tag{\pref{eq:linear-Q_expectation}} \\
        &=  \order\left(\epsilon H^2\right).
    \end{align*}
    Similarly, one can show $\E_t\left[\Qht_t(x,a) - Q^{\pi_t}_t(x,a)\right] = \order\left(\epsilon H^2\right)$. Summing them up over $t,x,a$ with weights $\qstar(x)\pistar(a|x)$ and $\qstar(x)\pi_t(a|x)$ respectively finishes the proof.  
\end{proof}

\begin{lemma}\label{lem: E.3 lemma}
    If $\eta \beta \leq \frac{\explore\lambda_{\min}}{24H^2\ln(\frac{1}{\epsilon\explore\lambda_{\min}})}$ and  $\eta\leq \frac{\explore\lambda_{\min}}{4H^2\ln(\frac{1}{\epsilon\explore\lambda_{\min}})}$, then $\E[\regterm]$ is upper bounded by
\begin{align*} 
    &\frac{H\ln |A|}{\eta} + 2\eta H^3\E\left[\sum_{t=1}^T \sum_{h=0}^{H-1}\sum_{(x,a)\in X_h\times A}\qstar(x)\pi_t(a|x)\|\phi(x,a)\|_{\hatcov_{t,h}}^2\right] 
    \\
    &\qquad \qquad + \frac{1}{H}\E\left[\sum_{t=1}^T \sum_{x,a}\qstar(x)\pi_t(a|x)\bonusQ_t(x,a)\right] + \otil\left(\eta\epsilon H^4 T + \frac{\eta H^4}{\explore^2\lambda_{\min}^2 T^2}\right).  
\end{align*}
\end{lemma}
\begin{proof}
    The proof is similar to that of \pref{lem: linear Q regret term}. 
        Again, we will apply the regret bound of the exponential weight algorithm \pref{lem: exponential weight lemma} for each state.  We start by checking the required condition: $\eta |\phi(x,a)^\top \hattheta_{\tau,h} - \bonusQ_t(x,a)|\leq 1$. This can be seen by
    \begin{align*}
        \eta \left|\phi(x,a)^\top \hattheta_{\tau, h}\right| 
        &= \eta \left| \phi(x,a)^\top \hatcov_{t,h} \phi(x_{t,h},a_{t,h})L_{t,h} \right| \times \left((1-Y_t) + Y_t \ind[h=h^*]H\right) \nonumber \\
        &\leq \eta \times \norm{\hatcov_{t,h}}_{\text{op}}\times L_{t,h} \times H  \nonumber \\ 
        &\leq \eta \times \frac{2}{\explore\lambda_{\min}}\ln \frac{1}{\epsilon\explore\lambda_{\min}} \times H^2 \tag{by \pref{lem: GR lemma contingency exploratory}} \\
        &\leq \frac{1}{2},  \tag{condition of the lemma}\\
        &   \label{eq: calculation of eta Q}
    \end{align*}
    and that by the definition of $\Bonus(t,x,a)$, we have 
    \begin{align}
        \eta\bonusQ_t(x,a) 
        &\leq \eta\times H\left(1+\frac{1}{H}\right)^H \times  2\beta\sup_{x,a,h} \|\phi(x,a)\|_{\hatcov_{t,h}}^2  \nonumber \\
        &\leq 6\eta \beta \times \frac{2H}{\explore\lambda_{\min}}\ln \frac{1}{\epsilon\explore\lambda_{\min}} \nonumber \tag{by \pref{lem: GR lemma contingency exploratory} again}\\
        &\leq \frac{1}{2H}, \label{eq: verfied 28}
    \end{align}
    where the last inequality is by the first condition of the lemma. 

    Thus, by \pref{lem: exponential weight lemma}, we have for any $x$, 
    \begin{align}
        &\E\left[\sum_{t=1}^T \sum_a \left(\pi_t(a|x) - \pistar(a|x)\right)\Qht_t(x,a)\right] \nonumber \\ 
        &\leq \frac{\ln |A|}{\eta } + 2\eta \E\left[\sum_{t=1}^T \sum_a  \pi_t(a|x)\Qht_t(x,a)^2\right] + 2\eta \E\left[\sum_{t=1}^T \sum_a  \pi_t(a|x)\bonusQ_t(x,a)^2\right]. \label{eq: regret Q tmp explore} 
    \end{align}
    The last term in \pref{eq: regret Q tmp explore} can be upper bounded by $ \E\left[\frac{1}{H}\sum_{t=1}^T \sum_a  \pi_t(a|x)\bonusQ_t(x,a)\right]$ because  $\eta \bonusQ_t(x,a)\leq  \frac{1}{2H}$ as we verified in \pref{eq: verfied 28}. To bound the second term in \pref{eq: regret Q tmp explore}, we use the following: for $(x,a)\in X_h\times A$, 
    \begin{align}
        &\E_t\left[\Qht_t(x,a)^2\right]  \nonumber \\
        &\leq H^2\E_t\left[\phi(x,a)^\top \hatcov_{t,h}\Big(((1-Y_t)+Y_t H \ind[h=h_t^*])^2\phi(x_{t,h}, a_{t,h})\phi(x_{t,h}, a_{t,h})^\top\Big) \hatcov_{t,h} \phi(x,a)\right]  \nonumber\\
        &= H^2\E_t\left[\phi(x,a)^\top \hatcov_{t,h}\Big((1-\explore)  \cov_{t,h} + \explore H \cov_{h}^{\pi_0} \Big) \hatcov_{t,h} \phi(x,a)\right]  \nonumber \\
        &\leq H^3\E_t\left[\phi(x,a)^\top \hatcov_{t,h}\cov_{t,h}^{\mix} \hatcov_{t,h} \phi(x,a)\right] \nonumber \\ 
        &\leq H^3\E_t\left[\phi(x,a)^\top \hatcov_{t,h}\cov_{t,h}^{\mix} (\cov_{t,h}^{\mix})^{-1}\phi(x,a)\right] + \otil\left(\epsilon H^3 + \frac{H^3}{\explore^2\lambda_{\min}^2 T^3}\right)   \tag{$*$}\\ 
        &= H^3\E_t\left[\|\phi(x,a)\|_{\hatcov_{t,h}}^2 \right] + \otil\left(\epsilon H^3 + \frac{H^3}{\explore^2\lambda_{\min}^2 T^3}\right),   \label{eq: followup}
    \end{align}    
    where $(*)$ is because by \pref{eq: GE 14} and \pref{eq: bounded norm prod exploratory}, $\norm{\hatcov_{t,h} -  (\cov_{t,h}^{\mix})^{-1}}_{\text{\rm op}} \leq 2\epsilon$ and 
        $\norm{\hatcov_{t,h}\cov_{t,h}^{\mix}}_{\text{\rm op}} \leq 1+2\epsilon$ hold with probability $1-\frac{1}{T^3}$; for the remaining probability, we upper bound $H^3\phi(x,a)^\top \hatcov_{t,h}\cov_{t,h}^{\mix} \hatcov_{t,h} \phi(x,a)$ by $\frac{4H^3}{\explore^2\lambda_{\min}^2}\ln^2\left(\frac{1}{\epsilon\explore\lambda_{\min}}\right)$ using \pref{eq: GE 13}. 
    
    Combining them with \pref{eq: regret Q tmp explore} and summing over states with weights $\qstar(x)$ finishes the proof. 
\end{proof}

Finally, we are ready to prove the regret bound.
\begin{proof}[Proof of \pref{thm:linear_Q_exploratory}]
Combining \pref{lem: mix algorithm bias term} and \pref{lem: E.3 lemma}, we see that if we choose $\beta=2\eta H^3$, then 
\begin{align*}
    &\E[\bias + \biastwo + \regterm] \\
    &\leq \otil\left(\frac{H}{\eta} + \epsilon H^3 T + \eta\epsilon H^4 T + \frac{\eta H^4}{\explore^2\lambda_{\min}^2 T^2}\right)  + \E\left[\sum_{t=1}^T \sum_{h=0}^{H-1}\sum_{(x,a)\in X_h\times A}\qstar(x)\pi_t(a|x)\bonus_t(x,a)\right] 
    \\
    &\qquad \qquad + \frac{1}{H}\E\left[\sum_{t=1}^T \sum_{x,a}\qstar(x)\pi_t(a|x)\bonusQ_t(x,a)\right].  
\end{align*}
%with $\bonusQ_t(x,a) = \bonus_t(x,a) + \left(1+\frac{1}{H}\right)\E_{x'\sim P(\cdot|x,a), a'\sim \pi_t(\cdot|x')}\bonusQ_t(x',a')$ and $\bonus_t(x,a)=\beta \|\phi(x,a)\|_{\hatcov_{t,h}}^2 +  \E_{j\sim \pi_t(\cdot|x)}\Big[\beta\|\phi(x,j)\|_{\hatcov_{t,h}}^2\Big]$ (see \pref{alg: generating B samples}). 
Hence, by \pref{lem: expected version}, we obtain the following bound, where we first set  $\epsilon = \frac{1}{H^4 T}$ so that all $\epsilon$-related terms are $\otil(1)$:
\begin{align}
    &\E\left[\sum_{t=1}^T V_t^{\pi_t}(x_0)\right] - \sum_{t=1}^T V_t^{\pistar}(x_0)   \nonumber\\
    &\leq  \otil\left(\frac{H}{\eta} + \frac{\eta H^4}{\explore^2\lambda_{\min}^2 T^2} + \E\left[\sum_{t=1}^T \sum_{x,a} q_t(x,a) \bonus_t(x,a) \right]\right)   \nonumber\\
    &\leq  \otil\left(\frac{H}{\eta} + \frac{\eta H^4}{\explore^2\lambda_{\min}^2 T^2}+ \beta\E\left[\sum_{t=1}^T \sum_{x,a} q_t(x,a) \|\phi(x,a)\|_{\hatcov_{t,h}}^2 \right]\right)    \nonumber\\
    &\leq  \otil\left(\frac{H}{\eta} + \frac{\eta H^4}{\explore^2\lambda_{\min}^2 T^2} + \beta\E\left[\sum_{t=1}^T \sum_{x,a} q_t(x,a) \|\phi(x,a)\|_{(\cov_{t,h}^{\mix})^{-1}}^2 \right]\right)    \nonumber \\
    &\leq  \otil\left(\frac{H}{\eta} + \frac{\eta H^4}{\explore^2\lambda_{\min}^2 T^2} + \frac{\beta}{1-\explore}\E\left[\sum_{t=1}^T \sum_{x,a} q_t(x,a) \|\phi(x,a)\|_{\cov_{t,h}^{-1}}^2 \right]\right)  \nonumber \\
    &\leq  \otil\left(\frac{H}{\eta} + \frac{\eta H^4}{\explore^2\lambda_{\min}^2 T^2} + \beta dHT\right) \tag{\pref{eq:LB_stability}} \\
    &= \otil\left(\frac{H}{\eta} + \frac{\eta H^4}{\explore^2\lambda_{\min}^2 T^2} + \eta dH^4T\right).  \tag{$\beta=2\eta H^3$}\\
    &   \label{eq: follow 3}
\end{align}
Since we explore with probability $\explore$, the final regret is 
\begin{align*}
    \E[\Reg] = \otil\left(\frac{H}{\eta} + \frac{\eta H^4}{\explore^2\lambda_{\min}^2 T^2} + \eta dH^4T + \explore HT\right). 
\end{align*}
Considering the constraints specified in \pref{lem: E.3 lemma}, we choose the parameters as follows: 
\begin{align*}
    \eta 
    &= \min\left\{ \frac{\explore\lambda_{\min}}{4H^2\ln(\frac{1}{\epsilon\explore\lambda_{\min}})}, \sqrt{\frac{\explore\lambda_{\min}}{48H^5\ln(\frac{1}{\epsilon\explore\lambda_{\min}})}} \right\}, \\
    \explore 
    &= \min\left\{\sqrt{\frac{H^2}{\lambda_{\min}T (\lambda_{\min} dH + 1)}}, \frac{1}{2}\right\}, \\
    \epsilon & = \frac{1}{H^4 T}.
\end{align*}
Then the regret can be bounded by $\order\left( \sqrt{H^5 dT} + H^2\sqrt{\frac{T}{\lambda_{\min}}} \right)$.
%\begin{align*}
    %\order\left(\sqrt{\frac{H^2}{\lambda_{\min}}\left(\lambda_{\min} dH^2 + 1\right)T}\right) = \order\left( \sqrt{H^5 dT} + H^2\sqrt{\frac{T}{\lambda_{\min}}} \right). 
%\end{align*}
\end{proof}

    %with the constraints $W=MN=\otil(\frac{1}{\epsilon^2\gamma^3})$ and $\frac{\eta \beta}{\gamma^2}\leq \order(1)$.
    %Choosing $\eta=\order(1/(Td^3H^2)^{\nicefrac{1}{4}})$, $\gamma=\order(1/(Td^3H^2)^{\nicefrac{1}{6}})$, and $\epsilon=\beta=\order(1/
    %(Td^3H^2)^{\nicefrac{1}{12}})$ gives the result.
