# Supplementary material for: Policy Optimization in Adversarial MDPs: Improved Exploration via Dilated Bonuses
Source: arXiv:2107.08346 source file (2021-07-18)
Supplement: Supplementary file 2 [file appendix-linearmdp-exploratory.tex]

\section{Details for Linear MDP with an Exploratory Policy}\label{app: linear MDP appendix} 

\begin{algorithm} 
    \caption{Policy Optimization with Dilated Bonuses (Linear MDP with an Exploratory Policy)}\label{alg:linearMDP}
    \textbf{Parameters}: $\lambda_{\min}, \beta, \eta, \epsilon$,  $M=\left\lceil\frac{96\ln(dHT)\ln^2(\frac{1}{\epsilon\explore\lambda_{\min}})}{\epsilon^2\explore^2\lambda_{\min}^2}\right\rceil$, $N=\left\lceil\frac{2}{\explore\lambda_{\min}}\ln \frac{1}{\epsilon \explore \lambda_{\min}}\right\rceil$, $\len=2MN$  \\ 
    \ \\
    \For{$k=1,2,\ldots, T/\len$}{
        \textbf{1) Interact with the environment}: Define $\pi_k$ as the following for $x\in X_h$:
        \begin{align}\label{eq:linear mdp policy}
            \pi_k(a|x) \propto \exp\left( -\eta \sum_{\tau=1}^{k-1} \left(\phi(x,a)^\top \hattheta_{\tau, h} - \phi(x,a)^\top\bonusVec_{\tau,h} - \bonus_\tau(x,a)\right) \right)  
        \end{align}
        where 
        \begin{align*}
            b_\tau(x,a) \triangleq \beta\|\phi(x,a)\|_{\hatcov_{\tau, h}}^2 + \beta \sum_{a'} \pi_\tau(a'|x)\|\phi(x,a')\|_{\hatcov_{\tau,h}}^2. 
        \end{align*}
        
        \ \\
        \ \\
        Randomly divide $[(k-1)\len+1, \ldots, k\len]$ into two parts: $S$ and $S'$, such that $|S|=|S'|=\len/2$. 
        \ \\
        \ \\

        \For{$t=(k-1)\len+1, \ldots, k\len$}{
            Draw $Y_t\sim \textsc{Bernoulli}(\explore)$.
            \\
            \lIf{$Y_t=1$ and $t\in S$}{
                Execute $\pi_0$
            }
            \ElseIf{$Y_t=1$ and $t\in S'$}{
                Draw $h_t^*\sim \text{Uniform}\{0, \ldots, H-1\}$. \\
                Execute $\pi_0$ in steps $0, \ldots, h_t^*-1$; continue with $\pi_t$ in steps $h_t^*, \ldots, H-1$. 
            }
            \lElse{Execute $\pi_t$}
            Collect trajectories $\{(x_{t,h}, a_{t,h}, \ell_t(x_{t,h},a_{t,h}))\}_{h=0}^{H-1}$ 
        }

        %where $\hatbonusQ_\tau(x,a)$ is an unbiased estimator of $\bonusQ_\tau(x,a)$ which is defined recursively as 
        %\begin{align*}            \bonusQ_\tau(x,a)\triangleq  \beta \|\phi(x,a)\|_{\hatcov_\tau}^2 + \E_{x',a'\sim \QQ_t(\cdot,\cdot|x,a)}\left[\beta \|\phi(x',a')\|_{\hatcov_\tau}^2 + \left(1+\frac{1}{H}\right) \bonusQ_\tau(x',a') \right]. 
        %\end{align*}
        \ \\
        \ \\
       
       \textbf{2) Construct inverse covariance matrix estimators:} 
       Use the samples in $S$ to calculate the following (note that $|S|=\len/2=MN$ and the $\GRMIX$ requires exactly $MN$ episodes of samples. We simply view these $MN$ episodes as calls within $\GRMIX$):  
       \begin{align}
           \left\{\hatcov_{k,h}\right\}_{h=0}^{H-1} = \GRMIX(k, M, N).  \label{eq: linear mdp gr}  
       \end{align}

       \textbf{3) Construct Q-function estimators: } Define for all $t,h$:
        \begin{align*}
            L_{t,h}&\triangleq \sum_{i=h}^{H-1}\ell_t(x_{t,i},a_{t,i})
        \end{align*}
        and
        \begin{align}
            \hattheta_{k,h}&\triangleq \hatcov_{k,h}\left(\frac{1}{|S'|}\sum_{t\in S'} ((1-Y_t) + Y_t H\ind[h=h_t^*]) \phi(x_{t,h},a_{t,h})L_{t,h} \right). \label{eq: theta estimator in linear MDP}
        \end{align}
        
        \textbf{4) Construct bonus function estimators: } Define for all $t,h$:
        \begin{align*} 
            D_{t,h}&\triangleq\left\{\begin{aligned}
          &0 &&\text{if $h=H-1$,}\\ &\sum_{i=h+1}^{H-1}\left(1+\frac{1}{H}\right)^{i-h} \bonus_{t}(x_{t,i}, a_{t,i})&&\text{otherwise;} \end{aligned}\right.
        \end{align*}
        and
        \begin{align}
             \bonusVec_{k,h}&\triangleq \hatcov_{k,h}\left( \frac{1}{|S'|}\sum_{t\in S'}((1-Y_t) + Y_t H\ind[h=h_t^*])\phi(x_{t,h},a_{t,h})D_{t,h} \right).
        \end{align} \label{eq: bonus function estimator in linear MDP}
    } 
\end{algorithm}

The algorithm for linear MDP with an exploratory policy $\pi_0$ is presented in \pref{alg:linearMDP}, which is based on the similar idea as \pref{alg: linear Q with exploratory}. Instead of changing policies on every episode, the algorithm proceeds in \emph{epochs}, each of which consists of $\len$ consecutive episodes, and the algorithm only updates its policy between epochs. We index epoch with $k$. The definitions of $\pi_k$, $\hatcov_{k,h}$, $\bonusQ_k(x,a)$ are analogous to those of $\pi_t$, $\hatcov_{t,h}$, $\bonusQ_t(x,a)$ in previous sections.

To deal with the epoch-based update, we define the following quantities (notice that the $k$-th epoch consists of episodes $(k-1)\len+1,\ldots, k\len$): 
\begin{definition}
\begin{align*}
    \barell_{k}(x,a) &\triangleq  \frac{1}{\len}\sum_{t=(k-1)\len+1}^{k\len}\ell_t(x,a) \\
    \barQ_{k}^{\pi}(x,a) &\triangleq  Q^{\pi}(x,a;\barell_k)\\
    \bartheta_{k,h}^{\pi} 
    &\triangleq  \frac{1}{\len}\sum_{t=(k-1)\len+1}^{k\len} \theta^{\pi}_{t,h} 
\end{align*}
\end{definition}

Recall that the main difference between \pref{alg:linearMDP} and \pref{alg: linear Q with exploratory} is that in \pref{alg:linearMDP} we use linear function approximation to calculate the bonus. The bonus $\bonusQ_k(x,a)$ and the \emph{estimated} bonus $\bonusVec_k(x,a)$ are defined in \pref{def: bonus for linear }.

\begin{definition}
    \label{def: bonus for linear }
    \begin{align*}
        \bonusQ_k(x,a) &\triangleq  \bonus_k(x,a) + \left(1+\frac{1}{H}\right)\E_{x'\sim P(\cdot|x,a)}\E_{a'\sim \pi_t(\cdot|x')}[\bonusQ_t(x',a')]  \tag{with $\bonusQ_k(x_H, a)\triangleq 0$} \\
        \hatbonusQ_k(x,a) &\triangleq \bonus_k(x,a) + \phi(x,a)^\top \bonusVec_{k,h}   \qquad \qquad \text{{\normalfont (for $x\in X_h$)}}
    \end{align*}
    where $\bonus_k(x,a)$ and $\bonusVec_{k,h}$ are defined in \pref{alg:linearMDP}.
\end{definition}

\subsection{Regret Analysis}
The regret decomposition for this section is slightly different from those in previous sections. Since we also use function approximation on the bonus $\bonusQ_t(x,a)$, we need to also account for its estimation error, resulting in two extra bias terms: 

\begin{align*}
	&\sum_{k=1}^{T/\len}\sum_x \qstar(x)\inner{\pi_k(\cdot|x)-\pistar(\cdot|x), \barQ^{\pi_k}_k(x,\cdot)-\bonusQ_k(x, \cdot)} \\ 
	&= \underbrace{\sum_{k=1}^{T/\len}\sum_x \qstar(x)\inner{\pi_k(\cdot|x), \barQ_k^{\pi_k}(x,\cdot)-\Qht_k(x,\cdot)}}_{\bias}+\underbrace{\sum_{k=1}^{T/\len}\sum_x\qstar(x)\inner{\pistar(\cdot|x), \Qht_k(x,\cdot)-\barQ_k^{\pi_k}(x,\cdot)}}_{\biastwo}\\
	&\quad +\underbrace{\sum_{k=1}^{T/\len}\sum_x\qstar(x)\inner{\pi_k(\cdot|x), \hatbonusQ_k(x,\cdot)-\bonusQ_k(x,\cdot)}}_{\biasthree}+\underbrace{\sum_{k=1}^{T/\len}\sum_x\qstar(x)\inner{\pistar(\cdot|x), \bonusQ_k(x,\cdot)-\hatbonusQ_k(x,\cdot)}}_{\biasfour}\\ 
	&\quad 
	 + \underbrace{\sum_{k=1}^{T/\len}\sum_x\qstar(x)\inner{\pi_k(\cdot|x)-\pistar(\cdot|x), \Qht_k(x,\cdot)-\hatbonusQ_k(x,\cdot)}}_{\regterm}
\end{align*}

In the following lemmas, we bound each term separately: 
\begin{lemma}
\label{lem: linear MDP bias term}
     \begin{align*}
         &\E[\bias + \biastwo] \leq \order\left(\frac{\epsilon H^3 T}{W}\right). 
     \end{align*}
\end{lemma} 
\begin{proof}   
    The proof of this lemma is almost identical to that of \pref{lem: mix algorithm bias term}, except that we replace $T$ by $T/\len$, and consider the averaged loss $\barell_k$ in an epoch instead of the single episode loss $\ell_t$: %Fix a $k\in [T/\len]$. Let $\overline{\ell}_k(\cdot,\cdot) = \frac{1}{\len}\sum_{t=(k-1)\len+1}^{k\len} \ell_t(\cdot,\cdot)$ and 
    %The following calculation is similar to \pref{eq: long proff 2}: 
    \begin{align}
        &\E_k\left[\barQ^{\pi_k}_k(x,a) - \Qht_k(x,a)\right]  \nonumber  \\
        &=\phi(x,a)^\top \left(\bartheta_{k,h}^{\pi_k} - \E_k\left[\hattheta_{k,h}\right]\right) \nonumber \\ 
        &= \phi(x,a)^\top \left(\bartheta_{k,h}^{\pi_k} - \E_k\left[\hatcov_{k,h}\right]\E_k\left[ \frac{1}{|S_k'|}\sum_{t\in S_k'} ((1-Y_t) + Y_t H\ind[h=h_t^*]) \phi(x_{t,h},a_{t,h})L_{t,h} \right]\right) \tag{$S_k'$ is the $S'$ in \pref{alg:linearMDP} within epoch $k$} \\
        &= \phi(x,a)^\top \left(\bartheta_{k,h}^{\pi_k} - \left( \cov_{k,h}^{\mix}\right)^{-1}\E_k\left[ \frac{1}{|S_k'|}\sum_{t\in S_k'} ((1-Y_t) + Y_t H\ind[h=h_t^*]) \phi(x_{t,h},a_{t,h})L_{t,h} \right]\right) + \order(\epsilon H^2) \tag{by \pref{lem: GR lemma contingency exploratory} and that $\|\phi(x,a)\|\leq 1$ for all $x,a$ and $L_{t,h}\leq H$} \\
        &=  \phi(x,a)^\top \left(\bartheta_{k,h}^{\pi_k} - \left( \cov_{k,h}^{\mix}\right)^{-1}\E_k\left[  \frac{1}{|S_k'|}\sum_{t\in S_k'}\cov_{k,h}^{\mix} \theta^{\pi_k}_{t,h} \right]\right)  + \order(\epsilon H^2)   \\
        &=  \phi(x,a)^\top \left(\bartheta_{k,h}^{\pi_k} - \left( \cov_{k,h}^{\mix}\right)^{-1}\E_k\left[  \frac{1}{\len}\sum_{t=(k-1)\len+1}^{k\len}\cov_{k,h}^{\mix} \theta^{\pi_k}_{t,h} \right]\right)  + \order(\epsilon H^2)  \tag{$S_k'$ is randomly chosen from epoch $k$}  \\  
        &= \phi(x,a)^\top \left(\bartheta_{k,h}^{\pi_k} - \left( \cov_{k,h}^{\mix}\right)^{-1}\cov_{k,h}^{\mix} \bartheta_{k,h}^{\pi_k}\right) + \order(\epsilon H^2) \nonumber \\
        &=\order\left(\epsilon H^2\right)    \label{eq: long proff 4}
    \end{align}
    Similarly, $\E_k\left[\Qht_k(x,a) - \barQ^{\pi_k}_k(x,a) \right] = \order\left(\epsilon H^2\right)$. Summing them over $k, x, a$ using weights $\qstar(x)\pi_k(a|x)$ and $\qstar(x)\pistar(a|x)$ respectively finishes the proof. 
\end{proof}

\begin{lemma}
\label{lem: linear MDP bias term}
     \begin{align*}
         &\E[\biasthree + \biasfour]\leq \otil\left( \frac{\epsilon H^3T}{W} \times \frac{\beta }{\explore\lambda_{\min}} \right). 
     \end{align*}
\end{lemma} 
\begin{proof}
    The proof is almost identical to that of the previous lemma. Recall the definition of $\Lambda_{k,h}^{\pi_k}$ in \pref{sec: linear MDP}. Then we have
    \begin{align} 
        &\E_k\left[\bonusQ_k(x,a) - \hatbonusQ_k(x,a)\right]  \nonumber  \\
        &=\phi(x,a)^\top \left(\Lambda_{k,h}^{\pi_k} - \E_k\left[\bonusVec_{k,h}\right]\right) \nonumber \\ 
        &= \phi(x,a)^\top \left(\Lambda_{k,h}^{\pi_k} - \E_k\left[\hatcov_{k,h}\right]\E_k\left[ \frac{1}{|S_k'|}\sum_{t\in S_k'} ((1-Y_t) + Y_t H\ind[h=h_t^*]) \phi(x_{t,h},a_{t,h})D_{t,h} \right]\right) \tag{$S_k'$ is the $S'$ in \pref{alg:linearMDP} within epoch $k$} \\
        &= \phi(x,a)^\top \left(\Lambda_{k,h}^{\pi_k} - \left( \cov_{k,h}^{\mix}\right)^{-1}\E_k\left[ \frac{1}{|S_k'|}\sum_{t\in S_k'} ((1-Y_t) + Y_t H\ind[h=h_t^*]) \phi(x_{t,h},a_{t,h})D_{t,h} \right]\right) \nonumber \\ 
        &\qquad \qquad \qquad \qquad + \otil\left(\epsilon H^2\times \frac{\beta}{\explore \lambda_{\min}}\right)  \tag{by \pref{lem: GR lemma contingency exploratory} and that $\|\phi(x,a)\|\leq 1$ for all $x,a$ and $D_{t,h}=\order(H\beta\sup\|\hatcov_{k,h}\|_{\text{op}})=\otil(\frac{H\beta}{\explore\lambda_{\min}})$} \\
        &=  \phi(x,a)^\top \left(\Lambda_{k,h}^{\pi_k} - \left( \cov_{k,h}^{\mix}\right)^{-1}\E_k\left[  \frac{1}{|S_k'|}\sum_{t\in S_k'}\cov_{k,h}^{\mix} \Lambda^{\pi_k}_{k,h} \right]\right)  + \otil\left(\epsilon H^2\times \frac{\beta}{\explore \lambda_{\min}}\right)  \nonumber \\
        &= \phi(x,a)^\top \left(\Lambda_{k,h}^{\pi_k} - \left( \cov_{k,h}^{\mix}\right)^{-1}\cov_{k,h}^{\mix} \Lambda_{k,h}^{\pi_k}\right) + \otil\left(\epsilon H^2\times \frac{\beta}{\explore \lambda_{\min}}\right) \nonumber \\
        &=\otil\left(\epsilon H^2\times \frac{\beta}{\explore \lambda_{\min}}\right).   
    \end{align}
    Similar for $\E_k[\hatbonusQ_k(x,a) - \bonusQ_k(x,a)]$. Summing them over $k, x, a$ using weights $\qstar(x)\pistar(a|x)$ and $\qstar(x)\pi_t(a|x)$ respectively /finishes the proof. 
\end{proof}

\begin{lemma}\label{lem: linear MDP regret term}
    Let $\frac{\eta \beta}{\explore^2\lambda_{\min}^2}\leq \frac{1}{160H^4 \ln(\frac{1}{\epsilon\explore\lambda_{\min}})^2}$ and $\frac{\eta}{\explore\lambda_{\min}}\leq \frac{1}{4H^2\ln(\frac{1}{\epsilon\explore\lambda_{\min}})}$. Then
    \begin{align*}
        &\E[\regterm]\\
        &=\otil\left(\frac{H}{\eta} + \frac{\eta\epsilon H^4T}{W} + \frac{\eta H^4}{\explore^2\lambda_{\min}^2 T^2W} + \frac{\eta \epsilon\beta^2 H^4T}{\explore^2\lambda_{\min}^2W} + \frac{\eta H^4\beta^2}{\explore^3\lambda_{\min}^3 T^2W}\right) \\
        &\qquad \qquad + 2\eta H^3\E\left[\sum_{k,x,a}\qstar(x)\pi_k(x,a)\|\phi(x,a)\|_{\hatcov_{k,h}}^2 \right]  + \frac{1}{H} \E\left[\sum_{k,x,a} \qstar(x)\pi_k(a|x)\bonusQ_k(x,a) \right]. 
    \end{align*}
\end{lemma}
\begin{proof}
    We first check the condition for \pref{lem: exponential weight lemma}: $\eta \left|\Qht_k(x,a) - \hatbonusQ_t(x,a)\right|\leq 1$. 
    In our case, 
    \begin{align*}
        \eta \left|\Qht_k(x,a)\right| 
        &= \eta \left| \phi(x,a)^\top \hatcov_{k,h}\left(\frac{1}{|S'|}\sum_{t\in S'} ((1-Y_t) + Y_t H\ind[h=h_t^*]) \phi(x_{t,h},a_{t,h})L_{t,h} \right) \right|  \\
        &\leq \eta \times \|\hatcov_{k,h}\|_{\text{op}}\times H \times \sup_{t\in S'} L_{t,h} \\
        &\leq \eta \times \frac{2}{\explore\lambda_{\min}}\ln \frac{1}{\epsilon\explore\lambda_{\min}} \times H^2 \tag{by \pref{lem: GR lemma contingency exploratory}} \\
        &\leq \frac{1}{2} \tag{by the condition specified in the lemma}
    \end{align*}
    and 
    \begin{align*}
        \eta\left|\hatbonusQ_k(x,a)\right| &\leq \eta \left|\bonus_k(x,a)\right| + \eta \left| \phi(x,a)^\top  \hatcov_{k,h}\left(\frac{1}{|S'|}\sum_{t\in S'} ((1-Y_t) + Y_t H\ind[h=h_t^*]) \phi(x_{t,h},a_{t,h})D_{t,h} \right) \right| \\
        &\leq \eta \times 2\beta \times \|\hatcov_{k,h}\|_{\text{op}} + \eta \times \|\hatcov_{k,h}\|_{\text{op}} \times  H \times \sup_{t\in S'} D_{t,h} \\
        &\leq \eta \times 2\beta \times \|\hatcov_{k,h}\|_{\text{op}} + \eta \times \|\hatcov_{k,h}\|_{\text{op}} \times  H \times (H-1)\left(1+\frac{1}{H}\right)^H  \times 2\beta \|\hatcov_{k,h}\|_{\text{op}}\\
        &\leq 8\eta \beta H^2\times \|\hatcov_{k,h}\|_{\text{op}}^2  \\
        &\leq 8\eta \beta H^2\left(\frac{2}{\explore\lambda_{\min}}\ln \frac{1}{\epsilon\explore\lambda_{\min}}\right)^2 \tag{by \pref{lem: GR lemma contingency exploratory}} \\
        &\leq \frac{1}{2H}.  \tag{by the condition specified in the lemma}
    \end{align*}
    
    An upper bound for $\E_k\left[\Qht_k(x,a)^2\right]$ follows the same calculation as in \pref{eq: followup}: 
    \begin{align}
        &\E_k\left[\Qht_k(x,a)^2\right]  \nonumber \\
        &\leq \E_k\left[\frac{1}{|S_k'|}\sum_{t\in S_k'}  H^2\phi(x,a)^\top \hatcov_{k,h}\Big(((1-Y_t)+Y_t H \ind[h=h_t^*])^2  \phi(x_{t,h}, a_{t,h})\phi(x_{t,h}, a_{t,h})^\top\Big) \hatcov_{k,h} \phi(x,a)\right]  \tag{$*$}\\ 
        %&\leq \frac{H^2}{|S'|^2}\E_k\left[\phi(x,a)^\top \hatcov_{k,h}\Big(((1-Y_t)+Y_t H \ind[h=h_t^*])^2\sum_{t,\tau\in S'}\phi(x_{t,h}, a_{t,h})\phi(x_{\tau,h}, a_{\tau,h})^\top\Big) \hatcov_{t,h} \phi(x,a)\right]  \nonumber\\
        &= \E_k\left[H^2\phi(x,a)^\top \hatcov_{k,h}\Big((1-\explore)  \cov_{k,h} + \explore H \cov_{h}^{\pi_0} \Big) \hatcov_{k,h} \phi(x,a)\right]  \nonumber \\
        &\leq H^3\E_k\left[\phi(x,a)^\top \hatcov_{k,h}\cov_{k,h}^{\mix} \hatcov_{k,h} \phi(x,a)\right] \nonumber \\ 
        &\leq H^3\E_k\left[\phi(x,a)^\top \hatcov_{k,h}\cov_{k,h}^{\mix} (\cov_{k,h}^{\mix})^{-1}\phi(x,a)\right] + \otil\left(\epsilon H^3 + \frac{H^3}{\explore^2\lambda_{\min}^2 T^3}\right)  \tag{by \pref{eq: GE 14} and \pref{eq: bounded norm prod exploratory}} \\ 
        &= H^3\E_k\left[\|\phi(x,a)\|_{\hatcov_{k,h}}^2 \right] + \otil\left(\epsilon H^3 + \frac{H^3}{\explore^2\lambda_{\min}^2 T^3}\right),   \label{eq: follow 2}
    \end{align}
    where in $(*)$ we use
    $\left(\frac{1}{|S_k'|}\sum_{t\in S_k'}v_t\right)^2\leq \frac{1}{|S_k'|}\sum_{t\in S_k'}v_t^2$ with $v_t = \phi(x,a)^\top \hatcov_{k,h}\left((1-Y_t) + Y_t H \ind[h=h_t^*]\right)\phi(x_{t,h}, a_{t,h})L_{t,h}$.

    Next, we bound $\E_t\left[\hatbonusQ_t(x,a)^2\right]$: 
    \begin{align*}
        &\E_k\left[\hatbonusQ_k(x,a)^2\right] \\
        &\leq 2\E_k\left[\bonus_k(x,a)^2\right] + 2\E_k\left[(\phi(x,a)^\top \bonusVec_{k,h})^2\right]\\
        &\leq 2\left(\beta \|\phi(x,a)\|_{\hatcov_{k,h}}^2 + \beta \E_{a'\sim \pi_k(\cdot|x)}\left[\|\phi(x,a')\|_{\hatcov_{k,h}}^2\right] \right)^2 \\
        &\qquad \quad + 2H^3 \left(\frac{6\beta}{\explore\lambda_{\min}}\ln\frac{1}{\epsilon\explore\lambda_{\min}}\right)^2\E_k\left[\|\phi(x,a)\|_{\hatcov_{k,h}}^2 \right] + \otil\left(\epsilon H^3 + \frac{H^3}{\explore^2\lambda_{\min}^2 T^3}\right)\times \left(\frac{6\beta}{\explore\lambda_{\min}}\ln\frac{1}{\epsilon\explore\lambda_{\min}}\right)^2 \\
        &\leq \frac{8\beta}{\explore\lambda_{\min}}\ln\frac{1}{\epsilon\explore\lambda_{\min}}\left(\beta  \|\phi(x,a)\|_{\hatcov_{k,h}}^2 + \beta \E_{a'\sim \pi_k(\cdot|x)}\left[\|\phi(x,a')\|_{\hatcov_{k,h}}^2\right] \right) \\
        &\qquad \quad + 2H^3 \left(\frac{6\beta}{\explore\lambda_{\min}}\ln\frac{1}{\epsilon\explore\lambda_{\min}}\right)^2\E_k\left[\|\phi(x,a)\|_{\hatcov_{k,h}}^2 \right] + \otil\left(\epsilon H^3 + \frac{H^3}{\explore^2\lambda_{\min}^2 T^3}\right)\times \left(\frac{6\beta}{\explore\lambda_{\min}}\ln\frac{1}{\epsilon\explore\lambda_{\min}}\right)^2 \\
        &\leq \left(\frac{8\beta}{\explore\lambda_{\min}}\ln\frac{1}{\epsilon\explore\lambda_{\min}} + \frac{72H^3\beta}{\explore^2\lambda_{\min}^2}\ln^2\left(\frac{1}{\epsilon\explore\lambda_{\min}}\right)\right)  \bonus_k(x,a) + \otil\left(\frac{\epsilon\beta^2 H^3}{\explore^2\lambda_{\min}^2} + \frac{H^3\beta^2}{\explore^4\lambda_{\min}^4 T^3}\right) \\
        &\leq  \frac{80H^3\beta}{\explore^2\lambda_{\min}^2}\ln^2\left(\frac{1}{\epsilon\explore\lambda_{\min}}\right)  \bonus_k(x,a) + \otil\left(\frac{\epsilon\beta^2 H^3}{\explore^2\lambda_{\min}^2} + \frac{H^3\beta^2}{\explore^4\lambda_{\min}^4 T^3}\right),
    \end{align*}
    where in the second inequality we bound $\E_k\left[(\phi(x,a)^\top \bonusVec_{k,h})^2\right]$ similarly as we bound $\E_k\left[\Qht_k(x,a)^2\right]$ in \pref{eq: follow 2}, except that we replace the upper bound for $L_{t,h}$ as $H$ by the upper bound for $D_{t,h}$ as $H\left(1+\frac{1}{H}\right)^H \beta\|\hatcov_{k,h}\|_{\text{op}} \leq 3H\times \beta\times \frac{2}{\explore\lambda_{\min}}\ln \frac{1}{\epsilon\explore\lambda_{\min}}$ by \pref{eq: GE 13}. In the third inequality, we use that 
    \begin{align*}
        \beta \|\phi(x,a)\|_{\hatcov_{k,h}}^2 \leq \beta \times \frac{2}{\explore\lambda_{\min}}\ln\frac{1}{\epsilon\explore\lambda_{\min}}. \tag{also by \pref{eq: GE 13}}
    \end{align*}
    
    Thus, by \pref{lem: exponential weight lemma}, we have 
    \begin{align*}
        &\E[\regterm] \\
        &\leq \otil\left(\frac{H}{\eta}\right) + 2\eta\sum_{k,x,a} \qstar(x)\pi_k(a|x) \Qht_k(x,a)^2 + 2\eta\sum_{k,x,a} \qstar(x)\pi_k(a|x) \bonusQ_k(x,a)^2 \\
        &\leq \otil\left(\frac{H}{\eta} + \frac{\eta\epsilon H^4T}{W} + \frac{\eta H^4}{\explore^2\lambda_{\min}^2 T^2W} + \frac{\eta \epsilon\beta^2 H^4T}{\explore^2\lambda_{\min}^2W} + \frac{\eta H^4\beta^2}{\explore^4\lambda_{\min}^4 T^2W}\right) \\
        &\qquad \qquad + 2\eta H^3\E\left[\sum_{k,x,a}\qstar(x)\pi_k(x,a)\|\phi(x,a)\|_{\hatcov_{k,h}}^2 \right] + \frac{160H^3\eta \beta}{\explore^2\lambda_{\min}^2}\ln^2\left(\frac{1}{\epsilon\explore\lambda_{\min}}\right) \E\left[\sum_{k,x,a} \qstar(x)\pi_k(a|x)\bonus_k(x,a) \right] \\
        &\leq \otil\left(\frac{H}{\eta} + \frac{\eta\epsilon H^4T}{W} + \frac{\eta H^4}{\explore^2\lambda_{\min}^2 T^2W} + \frac{\eta \epsilon\beta^2 H^4T}{\explore^2\lambda_{\min}^2W} + \frac{\eta H^4\beta^2}{\explore^4\lambda_{\min}^4 T^2W}\right) \\
        &\qquad \qquad + 2\eta H^3\E\left[\sum_{k,x,a}\qstar(x)\pi_k(x,a)\|\phi(x,a)\|_{\hatcov_{k,h}}^2 \right]  + \frac{1}{H} \E\left[\sum_{k,x,a} \qstar(x)\pi_k(a|x)\bonusQ_k(x,a) \right] 
    \end{align*}
    where in the last inequality we use the condition specified in the lemma and that $\bonusQ_k(x,a)\geq \bonus_k(x,a)$. 
    
\end{proof}

\begin{proof}[Proof of \pref{thm: linear MDP theorem}]
Now we combine the bounds in \pref{lem: linear MDP bias term}, \pref{lem: linear MDP bias term}, \pref{lem: linear MDP regret term}. We get  
\begin{align*}
    &\E[\bias + \biastwo + \biasthree + \biasfour + \regterm] \\
    &= \otil\left(\frac{H}{\eta} + \frac{\eta\epsilon H^4T}{W} + \frac{\eta H^4}{\explore^2\lambda_{\min}^2 T^2W} + \frac{\eta \epsilon\beta^2 H^4T}{\explore^2\lambda_{\min}^2W} + \frac{\eta H^4\beta^2}{\explore^4\lambda_{\min}^4 T^2W} + \frac{\epsilon H^3T}{W} \times \frac{\beta }{\explore\lambda_{\min}} + \frac{\epsilon H^3T}{W} \right)  \\
    &\qquad \qquad +  \sum_{k,x,a}\qstar(x)\pi_k(a|x)\bonus_k(x,a) \\
    &\qquad \qquad + \frac{1}{H}\sum_{k,x,a}\qstar(x)\pi_k(a|x)\bonusQ_k(x,a)
\end{align*}
where we use $\bonus_k=2\eta H^3$. By picking $\beta \leq \explore \lambda_{\min}$, the first term above can be further upper bounded by 
\begin{align*}
    \otil\left(\frac{H}{\eta} + \frac{\eta\epsilon H^4T}{W} + \frac{\eta H^4}{\explore^2\lambda_{\min}^2 T^2W} + \frac{\epsilon H^3T}{W} \right).
\end{align*}

By \pref{lem: expected version}, we have 

\begin{align*}
    &\E\left[\sum_{k=1}^{T/\len} V^{\pi_k}(x_0; \barell_k)\right] - \sum_{k=1}^{T/\len} V^{\pistar}(x_0; \barell_k) \\
    &\leq  \otil\left(\frac{H}{\eta} + \frac{\eta\epsilon H^4T}{W} + \frac{\eta H^4}{\explore^2\lambda_{\min}^2 T^2W} + \frac{\epsilon H^3T}{W} + \beta\E\left[\sum_{k=1}^{T/\len} \sum_{x,a} q_k(x)\pi_k(a|x) \|\phi(x,a)\|_{\hatcov_{k,h}}^2 \right]\right) \\
    &= \otil\left(\frac{H}{\eta} + \frac{\eta\epsilon H^4T}{W} + \frac{\eta H^4}{\explore^2\lambda_{\min}^2 T^2W} + \frac{\epsilon H^3T}{W} + \frac{\beta dH T}{\len}\right) \tag{by similar calculation as in \pref{eq: follow 3}} \\
    &= \otil\left(\frac{H}{\eta} + \frac{\eta\epsilon H^4T}{W} + \frac{\eta H^4}{\explore^2\lambda_{\min}^2 T^2W} + \frac{\epsilon H^3T}{W} + \frac{\eta dH^4 T}{\len}\right)   \tag{$\beta=2\eta H^3$}
\end{align*}

Multiplying back with $\len$, and considering the exploration rate $\explore$, we see that the true expected regret is upper bounded by
\begin{align*}
    &\otil\left(\frac{H\len}{\eta} + \eta\epsilon H^4T + \frac{\eta H^4}{\explore^2\lambda_{\min}^2 T^2} + \epsilon H^3T + \eta dH^4 T + \explore HT\right) \\
    &=\otil\left(\frac{H}{\eta \epsilon^2 \explore^3 \lambda_{\min}^3} + \eta\epsilon H^4T + \frac{\eta H^4}{\explore^2\lambda_{\min}^2 T^2} + \epsilon H^3T + \eta dH^4 T + \explore HT\right)
\end{align*}
where we use the specified value of $M$ and $N$ and that $\len=2MN$. 

Considering the constraints in \pref{lem: linear MDP regret term} and that $\beta=2\eta H^3$, we pick 
\begin{align*}
    \eta = \frac{\explore \lambda_{\min}}{20 H^{3.5} \ln\left(\frac{1}{\epsilon \explore \lambda_{\min}}\right)}
\end{align*}
which also makes $\beta\leq \explore\lambda_{\min}$ as we assumed previously. 

With this $\eta$, the regret can be simplified as 
\begin{align*}
    &\otil\left(\frac{H^{4.5}}{ \epsilon^2 \explore^4 \lambda_{\min}^4} + \explore\lambda_{\min}\epsilon \sqrt{H}T + \frac{ \sqrt{H}}{\explore\lambda_{\min} T^2} + \epsilon H^3T + \explore\lambda_{\min} d\sqrt{H} T + \explore HT\right) \\
    &=\otil\left(\frac{H^{4.5}}{ \epsilon^2 \explore^4 \lambda_{\min}^4} +  \epsilon H^3T + \explore\lambda_{\min} d\sqrt{H} T + \explore HT\right)
\end{align*}
By picking  
\begin{align*}
    \epsilon &= \left(\frac{H^{1.5}}{\explore^4\lambda_{\min}^4 T}\right)^{\frac{1}{3}},  \qquad \explore = \left(\frac{H^9}{T\lambda_{\min}^4(\lambda_{\min}d + \sqrt{H})^3}\right)^{\frac{1}{7}},  
\end{align*}
we get a regret bound of 
\begin{align*}
    \otil\left(\left(H^{12.5}\left(\frac{d\lambda_{\min} + \sqrt{H}}{\lambda_{\min}}\right)^4 T^6\right)^{\frac{1}{7}}\right). 
\end{align*}

\end{proof}
