# Supplementary material for: Policy Optimization in Adversarial MDPs: Improved Exploration via Dilated Bonuses
Source: arXiv:2107.08346 source file (2021-07-18)
Supplement: Supplementary file 3 [file appendix-linearmdp-backup.tex]

\section{Details Omitted in \pref{sec: linear MDP}}\label{app: linear MDP appendix}

\begin{algorithm}
    \caption{Policy Optimization with Dilated Bonuses in the Linear MDP case}\label{alg:linearMDP}
    \textbf{Parameters}: $\gamma, \beta, \eta, \epsilon$,  $M=\left\lceil\frac{24\ln(dHT)}{\epsilon^2\gamma^2}\right\rceil$, $N=\left\lceil\frac{2}{\gamma}\ln \frac{1}{\epsilon \gamma}\right\rceil$, $\len=2MN$  \\ 
    (for simplicity, assume that $M, N$ are integers) \\
    \ \\
    \For{$k=1,2,\ldots, T/\len$}{
        \textbf{1) Interact with the environment}: Execute $\pi_k$, which, for $x\in X_h$, is defined as 
        \begin{align}\label{eq:linear mdp policy}
            \pi_k(a|x) \propto \exp\left( -\eta \sum_{\tau=1}^{k-1} \phi(x,a)^\top \hattheta_{\tau, h} + \eta\sum_{\tau=1}^{k-1} B_{\tau}(x,a) \right)  
        \end{align}
        in episodes $(k-1)\len+1, \ldots, k\len$, 
        where $B_{\tau}(x,a)\triangleq\phi(x,a)^\top \bonusVec_{\tau, h} + \bonus_\tau(x,a)$ and 
        \begin{align*}
            b_\tau(x,a) \triangleq \beta\|\phi(x,a)\|_{\hatcov_{\tau, h}}^2 + \beta \sum_{a'} \pi_\tau(a'|x)\|\phi(x,a')\|_{\hatcov_{\tau,h}}^2. 
        \end{align*}
        
        
        Collect trajectories $\{(x_{t,h}, a_{t,h}, \ell_t(x_{t,h},a_{t,h}))\}_{h=0}^{H-1}$ for $t=(k-1)\len+1,\ldots, k\len$. 
        %where $\hatbonusQ_\tau(x,a)$ is an unbiased estimator of $\bonusQ_\tau(x,a)$ which is defined recursively as 
        %\begin{align*}            \bonusQ_\tau(x,a)\triangleq  \beta \|\phi(x,a)\|_{\hatcov_\tau}^2 + \E_{x',a'\sim \QQ_t(\cdot,\cdot|x,a)}\left[\beta \|\phi(x',a')\|_{\hatcov_\tau}^2 + \left(1+\frac{1}{H}\right) \bonusQ_\tau(x',a') \right]. 
        %\end{align*}
        \ \\
        \ \\
       Randomly divide $[(k-1)\len+1, \ldots, k\len]$ into two parts: $S$ and $S'$, such that $|S|=|S'|=\len/2$. 
       \ \\
       \ \\
       \textbf{2) Construct covariance matrix estimators:} 
       Use the samples in $S$ to calculate the following (note that $|S|=\len/2=MN$):  
       \begin{align}
           \left\{\hatcov_{k,h}\right\}_{h=0}^{H-1} = \GR(k, M, N, \gamma).  \label{eq: linear mdp gr}  
       \end{align}
       
        
       \textbf{3) Construct Q-function estimators: } Define for all $t,h$:
        \begin{align*}
            L_{t,h}&\triangleq \sum_{i=h}^{H-1}\ell_t(x_{t,i},a_{t,i})
        \end{align*}
        and
        \begin{align}
            \hattheta_{k,h}&\triangleq \hatcov_{k,h}\left(\frac{1}{|S'|}\sum_{t\in S'} \phi(x_{t,h},a_{t,h})L_{t,h} \right). \label{eq: theta estimator in linear MDP}
        \end{align}
        
        \textbf{4) Construct bonus function estimators: } Define for all $t,h$:
        \begin{align*} 
            D_{t,h}&\triangleq\left\{\begin{aligned}
          &0 &&\text{if $h=H-1$,}\\ &\sum_{i=h+1}^{H-1}\left(1+\frac{1}{H}\right)^{i-h} \bonus_{t}(x_{t,i}, a_{t,i})&&\text{otherwise;} \end{aligned}\right.
        \end{align*}
        and
        \begin{align}
             \bonusVec_{k,h}&\triangleq \hatcov_{k,h}\left( \frac{1}{|S'|}\sum_{t\in S'}\phi(x_{t,h},a_{t,h})D_{t,h} \right).
        \end{align} \label{eq: bonus function estimator in linear MDP}
    } 
\end{algorithm}

Define the following quantities: 
\begin{definition}
\begin{align*}
    \barell_{k}(x,a) &\triangleq  \frac{1}{\len}\sum_{t=(k-1)\len+1}^{k\len}\ell_t(x,a) \\
    \barQ_{k}^{\pi}(x,a) &\triangleq  Q^{\pi}(x,a;\barell_k)\\
    \bartheta_{k,h}^{\pi} 
    &\triangleq  \frac{1}{\len}\sum_{t=(k-1)\len+1}^{k\len} \theta^{\pi}_{t,h} 
\end{align*}
\end{definition}
\begin{definition}
    \begin{align*}
        \bonusQ_k(x,a) &= \bonus_k(x,a) + \left(1+\frac{1}{H}\right)\E_{x'\sim P(\cdot|x,a)}\E_{a'\sim \pi_t(\cdot|x')}[\bonusQ_t(x',a')] \\
        \hatbonusQ_k(x,a) &= \bonus_k(x,a) + \phi(x,a)^\top \bonusVec_{k,h}   \qquad \qquad \text{{\normalfont (for $x\in X_h$)}}
    \end{align*}
\end{definition}
 

\subsection{Regret Analysis}


\begin{align*}
	&\sum_{k=1}^{T/\len}\int \mathrm{d}\qstar(x)\inner{\pi_k(\cdot|x)-\pistar(\cdot|x), \barQ^{\pi_k}_k(x,\cdot)-\bonusQ_k(x, \cdot)} \\ 
	&= \underbrace{\sum_{k=1}^{T/\len}\int \mathrm{d}\qstar(x)\inner{\pi_k(\cdot|x), \barQ_k^{\pi_k}(x,\cdot)-\Qht_k(x,\cdot)}}_{\bias}+\underbrace{\sum_{k=1}^{T/\len}\int \mathrm{d}\qstar(x)\inner{\pistar(\cdot|x), \Qht_k(x,\cdot)-\barQ_k^{\pi_k}(x,\cdot)}}_{\biastwo}\\
	&\quad +\underbrace{\sum_{k=1}^{T/\len}\int \mathrm{d}\qstar(x)\inner{\pi_k(\cdot|x), \hatbonusQ_k(x,\cdot)-\bonusQ_k(x,\cdot)}}_{\biasthree}+\underbrace{\sum_{k=1}^{T/\len}\int \mathrm{d}\qstar(x)\inner{\pistar(\cdot|x), \bonusQ_k(x,\cdot)-\hatbonusQ_k(x,\cdot)}}_{\biasfour}\\ 
	&\quad 
	 + \underbrace{\sum_{k=1}^{T/\len}\int \mathrm{d}\qstar(x)\inner{\pi_k(\cdot|x)-\pistar(\cdot|x), \Qht_k(x,\cdot)-\hatbonusQ_k(x,\cdot)}}_{\regterm}
\end{align*}

\begin{lemma}
\label{lem: linear MDP bias term}
     \begin{align*}
         &\E[\bias + \biastwo]\\
         &\leq \frac{\beta}{4} \E\left[\sum_{k=1}^{T/\len} \sum_{h=0}^{H-1} \int_{x\in X_h} \de\qstar(x) \sum_a (\pi_k(a|x)+\pistar(a|x)) \|\phi(x,a)\|_{\hatcov_{k,h}}^2\right]  +  \order\left(\frac{\gamma dH^3T}{\beta \len} + \frac{\epsilon H^2T}{\len}\right). 
     \end{align*}
\end{lemma} 
\begin{proof}
    The proof of this lemma is almost identical to that of \pref{lem: linear Q bias term}, except that we replace $T$ by $T/\len$, and consider the averaged loss $\barell_k$ in an epoch instead of the single episode loss $\ell_t$. %Fix a $k\in [T/\len]$. Let $\overline{\ell}_k(\cdot,\cdot) = \frac{1}{\len}\sum_{t=(k-1)\len+1}^{k\len} \ell_t(\cdot,\cdot)$ and 
    The following calculation is similar to \pref{eq: long proff 2}: 
    \begin{align}
        &\E_k\left[\barQ^{\pi_k}_k(x,a) - \Qht_k(x,a)\right]  \nonumber  \\
        &=\phi(x,a)^\top \left(\bartheta_{k,h}^{\pi_k} - \E_k\left[\hattheta_{k,h}\right]\right) \nonumber \\ 
        &= \phi(x,a)^\top \left(\bartheta_{k,h}^{\pi_k} - \E_k\left[\hatcov_{k,h}\right]\E_k\left[ \frac{1}{|S_k'|}\sum_{t\in S_k'}\phi(x_{t,h},a_{t,h})L_{t,h} \right]\right) \tag{$S_k'$ is the $S'$ in \pref{alg:linearMDP} within epoch $k$} \\
        &=  \phi(x,a)^\top \left(\bartheta_{k,h}^{\pi_k} - \left(\gamma I + \cov_{k,h}\right)^{-1}\E_k\left[  \frac{1}{|S_k'|}\sum_{t\in S_k'}\phi(x_{t,h},a_{t,h})L_{t,h} \right]\right)  + \order(\epsilon H)  \tag{by \pref{lem: GR lemma contingency} and that $\|\phi(x,a)\|\leq 1$ for all $x,a$ and $L_{t,h}\leq H$} \\
        &=  \phi(x,a)^\top \left(\bartheta_{k,h}^{\pi_k} - \E_k\left[\frac{1}{\len}\sum_{t=(k-1)\len+1}^{k\len}\left(\gamma I + \cov_{k,h}\right)^{-1}  \phi(x_{t,h},a_{t,h})\phi(x_{t,h},a_{t,h})^\top \theta_{t,h}^{\pi_k} \right]\right)  + \order(\epsilon H) \tag{$S_k'$ is randomly chosen from epoch $k$}  \\
        &= \phi(x,a)^\top \left(\bartheta_{k,h}^{\pi_k} - \left(\gamma I + \cov_{k,h}\right)^{-1}\cov_{k,h} \bartheta_{k,h}^{\pi_k}\right) + \order(\epsilon H) \nonumber \\
        &= \gamma  \phi(x,a)^\top (\gamma I + \cov_{k,h})^{-1} \bartheta_{k,h}^{\pi_k}+ \order(\epsilon H)\nonumber \\
        %&= \gamma \E_t\left[ \phi(x,a)^\top \hatcov_t \theta_t^{\pi_t}\right]+ \order\left(\epsilon \left(H^2 + \gamma \sqrt{d}H\right)\right) \nonumber \\
        &\leq \frac{\beta}{4}  \|\phi(x,a)\|_{(\gamma I + \cov_{k,h})^{-1}}^2  + \frac{\gamma^2}{\beta}  \|\bartheta_{k,h}^{\pi_k}\|_{(\gamma I + \cov_{k,h})^{-1}}^2 + \order(\epsilon H) \nonumber \\
        &\leq \frac{\beta}{4} \E_t\left[  \|\phi(x,a)\|_{\hatcov_{k,h}}^2\right] + \frac{\gamma dH^2}{\beta} + \order\left(\epsilon (H+\beta)\right)    \label{eq: long proff 4}
    \end{align}
\end{proof}


\begin{lemma}
\label{lem: linear MDP bias term}
     \begin{align*}
         &\E[\biasthree + \biasfour]\\
         &\leq \frac{\beta}{4} \E\left[\sum_{k=1}^{T/\len} \sum_{h=0}^{H-1} \int_{x\in X_h} \de\qstar(x) \sum_a (\pi_k(a|x)+\pistar(a|x)) \|\phi(x,a)\|_{\hatcov_{k,h}}^2\right]  +  \order\left(\frac{\gamma dH^3T}{\beta \len} + \frac{\epsilon H^2T}{\len}\right). 
     \end{align*}
\end{lemma} 
\begin{proof}
    The following calculation is similar to \pref{eq: long proff 4}: 
    \begin{align}
        &\E_k\left[\bonusQ_k(x,a) - \hatbonusQ_k(x,a)\right]  \nonumber  \\
        &=\phi(x,a)^\top \left(\Lambda_{k,h}^{\pi_k} - \E_k\left[\bonusVec_{k,h}\right]\right) \nonumber \\  
        &= \phi(x,a)^\top \left(\Lambda_{k,h}^{\pi_k} - \E_k\left[\bonusVec_{k,h}\right]\E_k\left[ \frac{1}{|S_k'|}\sum_{t\in S_k'}\phi(x_{t,h},a_{t,h})D_{t,h} \right]\right) \\
        &=  \phi(x,a)^\top \left(\Lambda_{k,h}^{\pi_k} - \left(\gamma I + \cov_{k,h}\right)^{-1}\E_k\left[  \frac{1}{|S_k'|}\sum_{t\in S_k'}\phi(x_{t,h},a_{t,h})D_{t,h} \right]\right)  + \order\left(\frac{\epsilon \beta H}{\gamma}\right)  \tag{by \pref{lem: GR lemma contingency} and that $\|\phi(x,a)\|\leq 1$ for all $x,a$ and $D_{t,h}= \order\left(\frac{\beta H}{\gamma}\right)$} \\
        &=  \phi(x,a)^\top \left(\Lambda_{k,h}^{\pi_k} - \E_k\left[  \frac{1}{\len}\sum_{t=(k-1)\len+1}^{k\len}\left(\gamma I +  \cov_{k,h}\right)^{-1}\phi(x_{t,h},a_{t,h})\phi(x_{t,h},a_{t,h})^\top \Lambda_{t,h}^{\pi_k} \right]\right)  + \order\left(\frac{\epsilon \beta H}{\gamma}\right) \nonumber \\
        &= \phi(x,a)^\top \left(\Lambda_{k,h}^{\pi_k} - \left(\gamma I + \cov_{k,h}\right)^{-1}\cov_{k,h} \Lambda_{k,h}^{\pi_k}\right) + \order\left(\frac{\epsilon \beta H}{\gamma}\right) \tag{$S_k'$ is randomly chosen from epoch $k$} \\
        &= \gamma  \phi(x,a)^\top (\gamma I + \cov_{k,h})^{-1} \Lambda_{k,h}^{\pi_k}+ \order(\epsilon H)\nonumber \\
        %&= \gamma \E_t\left[ \phi(x,a)^\top \hatcov_t \theta_t^{\pi_t}\right]+ \order\left(\epsilon \left(H^2 + \gamma \sqrt{d}H\right)\right) \nonumber \\
        %& \leq \gamma \|\phi(x,a)\|_{(\gamma I + \cov_{k,h})^{-1}} \|\Lambda_{k,h}^{\pi_k}\|_{_{(\gamma I + \cov_{k,h})^{-1}}}  \\
        %& \lesssim  \|\phi(x,a)\|_{(\gamma I + \cov_{k,h})^{-1}} \times \frac{\beta}{\gamma} \tag{because $\|\Lambda_{k,h}^{\pi_k}\|\lesssim \frac{\beta}{\gamma}$} \\ 
        &\leq \frac{\beta}{4}  \|\phi(x,a)\|_{(\gamma I + \cov_{k,h})^{-1}}^2  + \frac{\gamma^2}{\beta}  \|\Lambda_{k,h}^{\pi_k}\|_{(\gamma I + \cov_{k,h})^{-1}}^2 + \order(\epsilon H) \nonumber \\
        &\leq \frac{\beta}{4} \E_t\left[  \|\phi(x,a)\|_{\hatcov_{k,h}}^2\right] + \frac{\gamma dH^2}{\beta} + \order\left(\epsilon (H+\beta)\right)    \label{eq: long proff 6}
    \end{align}
\end{proof}




\begin{lemma}\label{lem: linear MDP regret term}
    Let $\frac{\eta \beta}{\gamma^2}\leq \frac{1}{3eH^2}$ and $\frac{\eta}{\gamma}\leq \frac{1}{8H}$. Then
    \begin{align*}
        \E[\regterm]&\leq \frac{H\ln |A|}{\eta} + 2\eta H \E\left[\sum_{k=1}^{T/M}\int\mathrm{d}\qstar(x)\sum_{a}\pi_k(a|x)\|\phi(x,a)\|_{\hatcov_k}^2\right]\\
        &\qquad +\frac{1}{H} \E\left[ \sum_{k=1}^{T/M} \int\mathrm{d}\qstar(x)\sum_{a}\pi_k(a|x)B_k(x,a) \right]+\order\left(\epsilon H^3T\right)   .
    \end{align*}
\end{lemma}
\begin{proof}
     The proof of this lemma is similar to the previous section except for the condition $\eta \left|\phi(x,a)^\top \hattheta_\tau - \bonusQ_t(x,a)\right|\leq 1$. 
    In the case, 
    \begin{align*}
        \eta \left|\phi(x,a)^\top \hattheta_\tau\right| 
        &= \eta \left| \phi(x,a)^\top \hatcov_t \left(\sum_{h}\phi(x_{t,h},a_{t,h})L_{t,h}\right) \right|  
        \leq \eta \times \left(\frac{1}{\gamma}+\epsilon\right)\times H \leq \frac{1}{2}
    \end{align*}
    and 
    \begin{align*}
        \eta\bonusQ_t(x,a) \leq \eta\beta \left(2+\frac{1}{H}\right)\frac{e}{\gamma^2}\times H\leq \frac{1}{H}\leq \frac{1}{2}.  
    \end{align*}
\end{proof}


\begin{lemma}\label{lem: linear MDP bonus term}
    \begin{align*}
        \E[\negterm] 
        &\leq \E\left[\sum_{k=1}^{T/M} \qstar(x_0)\pi_k(a|x_0)\bonusQ_k(x_0,a)\right] \\
        &\qquad - \beta\E\left[\sum_{k=1}^{T/M} \sum_{h>0}\sum_{(x,a)\in X_h\times A}\qstar(x)\pi_k(a|x)\left(\|\phi(x,a)\|_{\hatcov_k}^2 + \frac{1}{H}\bonusQ_k(x,a)\right)\right] \\
        &\qquad - 
        \beta\E\left[\sum_{k=1}^{T/M} \sum_{h\geq 0}\sum_{(x,a)\in X_h\times A}\qstar(x)\pistar(a|x)\|\phi(x,a)\|_{\hatcov_k}^2\right]
    \end{align*}
\end{lemma}
\begin{proof}
    The proof of this lemma is similar to the previous section.
\end{proof}

\begin{comment}
\begin{proof}
    By the definition of $\bonusQ_t(x,a)$, for $(x,a)\in X_h\times A$ with $h<H-1$, we have
    \begin{align*}
        \E\left[\bonusQ_t(x,a)\right] 
        &=\beta\|\phi(x,a)\|_{\hatcov_t}^2 + \E_{x'\sim p(\cdot|x,a), a'\sim \pi_t(\cdot|x')}\left[\beta\|\phi(x',a')\|_{\hatcov_t}^2+ \left(1+\frac{1}{H}\right) \bonusQ_t(x',a') \right], 
    \end{align*}
    and $\E[\bonusQ_t(x,a)]=\beta\|\phi(x,a)\|_{\hatcov_t}^2$ for $(x,a)\in X_{H-1}\times A$. 
    
    Below, we define $\bonus_t(x,a) = \beta\|\phi(x,a)\|_{\hatcov_t}^2$. 
    
    For a single layer $h<H-1$,  
    \begin{align*}
        &\E\left[\sum_{x\in X_h}\sum_{a\in A}\qstar(x)\left(\pi_t(a|x) - \pistar(a|x)\right)\bonusQ_t(x,a)\right]\\
        &= \E\left[\sum_{x\in X_h}\sum_{a\in A}\qstar(x)\pi_t(a|x)\bonusQ_t(x,a)\right] - \E\left[\sum_{x\in X_h}\sum_{a\in A} \qstar(x)\pistar(a|x)\bonusQ_t(x,a)\right]\\
        &= \E\left[\sum_{x\in X_h}\sum_{a\in A}\qstar(x)\pi_t(a|x)\bonusQ_t(x,a)\right] - \E\left[\sum_{x\in X_h}\sum_{a\in A}\qstar(x)\pistar(a|x)\bonus_t(x,a)\right] \\
        &\qquad \qquad - \E\left[\sum_{x\in X_h}\sum_{a\in A} \qstar(x)\pistar(a|x)\E_{x'\sim p(\cdot|x,a)}\E_{a'\sim \pi_t(\cdot|x')}\left[\bonus_t(x',a') + \left(1+\frac{1}{H}\right)\bonusQ_t(x',a')\right]\right]\\
        &\leq \E\left[\sum_{x\in X_h}\sum_{a\in A}\qstar(x)\pi_t(a|x)\bonusQ_t(x,a)\right] - \E\left[\sum_{x'\in X_{h+1}}\sum_{a'\in A} \qstar(x')\pi_t(a'|x')\bonusQ_t(x',a')\right] \\
        &\qquad \qquad - \E\left[\sum_{x\in X_h}\sum_{a\in A}\qstar(x)\pistar(a|x)\bonus_t(x,a)\right] - \E\left[\sum_{x'\in X_{h+1}}\sum_{a'\in A} \qstar(x')\pi_t(a'|x')\left(\bonus_t(x',a') + \frac{1}{H}\bonusQ_t(x',a')\right)\right]. 
    \end{align*}
    
    
    Summing the above inequality over $h=0, \ldots, H-2$, performing telescoping, and adding  $\E\left[\sum_{x\in X_{H-1}}\sum_{a\in A} \qstar(x)(\pi_t(a|x)- \pistar(a|x))\bonusQ_t(x,a)\right]$, we get the desired inequality. 
    
    %\begin{align*}
    %    \E[\negterm] 
    %    &\leq \E\left[\sum_{t=1}^T \qstar(x_0)\pi_t(a|x_0)\bonusQ_t(x_0,a)\right] \\
    %    &\qquad - \E\left[\sum_{t=1}^T \sum_{h=1}^{H-1}\sum_{(x,a)\in X_h\times A}\qstar(x)\pi_t(a|x)\left(\bonus_t(x,a) + \frac{1}{H}\bonusQ_t(x,a)\right)\right] \\
    %    &\qquad - 
    %    \E\left[\sum_{t=1}^T \sum_{h= 0}^{H-1}\sum_{(x,a)\in X_h\times A}\qstar(x)\pistar(a|x)\bonus_t(x,a)\right]
    %\end{align*}
\end{proof}

\end{comment}


\begin{lemma}
    \begin{align*}
        \E[\Reg] \leq \otil\left(H^{\nicefrac{17}{6}}d^{\nicefrac{3}{4}}T^{\nicefrac{11}{12}}\right) 
    \end{align*}
\end{lemma}

\begin{proof}
Now we combine the bounds in \pref{lem: linear MDP bias term}, \pref{lem: linear MDP regret term}, \pref{lem: linear MDP bonus term}. We get that under the constraints $\frac{\eta \beta}{\gamma^2}\leq \frac{1}{3eH^2}$ and $\frac{\eta}{\gamma}\leq \frac{1}{8H}$ and $\beta > 4\eta H$, we have 
\begin{align*}
    &\E[\Reg]\\
    &\le W\cdot\E\left[\bias + \biastwo + \regterm + \negterm \right]\\
    &\leq W\cdot \order\left( \frac{H\ln |A|}{\eta} + \frac{\gamma dH^3T}{\beta W} + \epsilon H^3\frac{T}{W} \right)\\
    &\leq  \otil\left( \frac{HW}{\eta} + \frac{\gamma dH^3T}{\beta} + \epsilon H^3 {T}  \right). 
\end{align*}

    with the constraints $W=MN=\otil(\frac{1}{\epsilon^2\gamma^3})$ and $\frac{\eta \beta}{\gamma^2}\leq \order(1)$.
    Choosing $\eta=\order(1/(Td^3H^2)^{\nicefrac{1}{4}})$, $\gamma=\order(1/(Td^3H^2)^{\nicefrac{1}{6}})$, and $\epsilon=\beta=\order(1/
    (Td^3H^2)^{\nicefrac{1}{12}})$ gives the result.
\end{proof}
